# Supplementary material for: Interference-Aware Edge Runtime Prediction with Conformal Matrix Completion
Source: arXiv:2503.06428 source file (2025-03-09)
Supplement: Supplementary file 1 [file artifact.tex]

\section{Artifact Appendix}

Our artifact implements the interference-aware conformal prediction algorithm described in this paper. Our implementation is GPU-accelerated (and tuned for 24-GB Nvidia GPUs) and parallelized using Jax, and includes a poetry lock file to install dependencies. The artifact provided includes code to (1) generate train/val/test splits, (2) train the experiments described in the paper, (3) summarize these experiments into key performance metrics, and (4) reproduce the figures shown in the paper. We also include our dataset, which is packaged with the repository. Finally, our splits, results, and summary metrics are archived to Zenodo.

In addition to an archived version of our repository and results on Zenodo (\url{https://zenodo.org/records/14977004}), our repository and dataset can also be found on Github (\url{https://github.com/wiseLabCMU/pitot}).

\subsection{Artifact check-list (meta-information)}

{\em Obligatory. Use just a few informal keywords in all fields applicable to your artifacts
and remove the rest. This information is needed to find appropriate reviewers and gradually 
unify artifact meta information in Digital Libraries.}

{\small
\begin{itemize}
  \item {\bf Algorithm: } matrix completion for program runtime prediction + extension for interference + extension for conformal prediction
  \item {\bf Run-time environment:} linux, cuda, python/conda
  \item {\bf Hardware: } Nvidia GPU, 24GB VRAM
  \item {\bf How much disk space required (approximately): } $<$5GB and a conda environment
  \item {\bf How much time is needed to prepare workflow (approximately)?: } $<$ 10 minutes
  \item {\bf How much time is needed to complete experiments (approximately)?: } $\approx$ 6-12 hours using a RTX 4090
  \item {\bf Publicly available?: } yes
  \item {\bf Code licenses (if publicly available)?: } MIT
  \item {\bf Data licenses (if publicly available)?: } MIT
  \item {\bf Archived (provide DOI)?: } 10.5281/zenodo.14977004
\end{itemize}
}

%%%%%%%%%%%%%%%%%%%%%%%%%%%%%%%%%%%%%%%%%%%%%%%%%%%%%%%%%%%%%%%%%%%%%
\subsection{Description}

\subsubsection{How to access}

Clone this repository, and follow the instructions listed: \url{https://github.com/wiseLabCMU/pitot}. Minimal disk space is required for the repository ($<$ 5GB after generating all outputs), though considerably more may be consumed by the python environment after installing dependencies if they are not already present.

\subsubsection{Hardware dependencies}

Nvidia GPU; 24GB VRAM (e.g., RTX 3090/4090)

\subsubsection{Software dependencies}

Linux, Conda, Poetry

\subsubsection{Data sets}

All data is included with the repository.

\subsection{Installation}

Conda create, poetry install, followed by an included makefile; see the README for exact commands.

\subsection{Experiment workflow}

The experiment workflow is documented in a Makefile; the make commands associated with each stage are documented in the README. Some commands in the Makefile such as training execution also use logic in the python training script to queue and batch training.

Evaluators may find it useful to use \texttt{nq} (\url{https://github.com/leahneukirchen/nq}) to easily queue multiple steps.

\subsection{Evaluation and expected result}

Follow instructions in the README. Our output (splits, results, summary) can be found on Zenodo (\url{https://zenodo.org/records/14977004}); note that due to floating point differences, non-deterministic RNG leaking into our experiments, etc, the results may not necessarily be numerically identical.

\subsection{Experiment customization}

The code is written in a modular structure with docstrings and type annotations, including \texttt{dtype} and \texttt{shape} annotations using \texttt{jaxtyping}. All tunable parameters are documented via these docstring annotations.
